# Supplementary material for: On-node lattices construction using $\textit{partial}$ Gauss-Hermite quadrature for the lattice Boltzmann method
Source: arXiv:1903.11959 ancillary file (2019-03-26)
Supplement: Supplementary file 1 [file SI.pdf]

# Supporting information for "On-node lattices construction using *partial* Gauss-Hermite quadrature for the lattice Boltzmann method"

Huanfeng Ye* and Bo Kuang
*School of Nuclear Science and Engineering, Shanghai Jiao Tong University, Shanghai 200240, China*

Zecheng Gan
*Department of Mathematics, University of Michigan, Ann Arbor, MI 48109-1043, USA*

Yanhua Yang
*School of Nuclear Science and Engineering, Shanghai Jiao Tong University, Shanghai 200240, China and National Energy Key Laboratory of Nuclear Power Software, Beijing 102209, China*

* E-mail address: huanfye@163.com

In Sec. I, we briefly revisit the derivation of the Hermite polynomial expansion. In Sec. II, we present the detailed derivation of the pGHQ theory. In Sec. III, we address the mathematical equivalence between the pGHQ scheme and the Shan scheme. In Sec. IV, we illustrate the mathematical equivalence between the pGHQ scheme and the Karlin-Asinari scheme on obtaining the lattice constant and weights.

## I. HERMITE POLYNOMIAL EXPANSION

The Hermite polynomial expansion we employed in the paper is a simplified version of Ref. [1] with constant temperature in whole fluid field. To demonstrate the mathematical mechanism behind the Hermite polynomial expansion, we derive it through a top-down approach instead of the original directly projecting BGK-Boltzmann equation into Hermite spectral space. The derivation is based on a unidimensional Maxwell distribution,

$$f\left(v\right)=\frac{\rho}{\sqrt{\pi 2RT}}e^{-\frac{\left(v-u\right)^{2}}{2RT}}, \tag{S1}$$

where $v$ and $u$ stands for micro and macro velocity respectively, $T$ is the temperature , $\rho$ is the density, and $R$ is the gas constant. We start with nondimensionalizing the moment equation of equilibrium distribution (ED) discretization,

$$\begin{aligned} M^{k} &= \int \frac{\rho}{\sqrt{\pi 2RT}}e^{-\frac{\left(v-u\right)^{2}}{2RT}}v^{k}dv \\ &= \left(\sqrt{2RT}\right)^{k}\int \frac{\rho}{\sqrt{\pi}}e^{-\left(\xi-\phi\right)^{2}}\xi^{k}d\xi \\ &= \left(\sqrt{2RT}\right)^{k}\sum_{\alpha=0}^{q-1} f_{\alpha}^{eq}\xi_{\alpha}^{k}, \end{aligned} \tag{S2}$$

by change of variable $\xi=v/\sqrt{2RT}$, $\phi=u/\sqrt{2RT}$. ED discretization is to construct an equilibrium distribution on a discrete velocity set which evaluates the above moment integral $M^k$ exactly. It involves two nomenclatures, abscissa number $q$ and moment degree $n$, which denote the number of discrete velocities and the highest retained degree of moment integral $M^k$ for the discretization respectively. With the constant temperature $T$ assumption, Eq. (S2) indicates that ED discretization can be performed on the dimensionless velocity $\xi$ with dimensionless Maxwellian moment integral $m^k=M^k/\left(\sqrt{2RT}\right)^k$, instead of the physical velocity $v$. The corresponding dimensionless Maxwell distribution is

$$g=\frac{\rho}{\sqrt{\pi}}e^{-\left(\xi-\phi\right)^{2}}. \tag{S3}$$

Expanding it with Hermite polynomials [2], the above distribution can be expressed as

$$g=\frac{\rho}{\sqrt{\pi}}e^{-\xi^{2}}\sum_{i=0}^{\infty}H_{i}\left(\xi\right)\frac{\phi^{i}}{i!}. \tag{S4}$$

It implies that the dimensionless Maxwellian moment integral of a given degree is solely determined by the Hermite terms up to that degree and not changed by the truncation of higher-degree terms,

$$m^{k}=\int g\xi^{k}d\xi=\int \frac{\rho}{\sqrt{\pi}}e^{-\xi^{2}}\sum_{i=0}^{k}H_{i}\left(\xi\right)\frac{\phi^{i}}{i!}\xi^{k}d\xi. \tag{S5}$$

Neglecting the effect of higher-degree Hermite term, then the discretization with moment degree $n$ can be converted into a $2n$-degree quadrature problem with weigh function $\exp\left(-\xi^{2}\right)$. The corresponding discrete equilibrium distribution is

$$f_{\alpha}^{eq}=\mathrm{w}_{\alpha}\rho\sum_{i=0}^{n}H_{i}\left(\xi_{\alpha}\right)\frac{\phi^{i}}{i!}, \tag{S6}$$

with

$$\rho=\sum_{\alpha=0}^{q-1} f_\alpha^{eq}, \quad \phi=\sum_{\alpha=0}^{q-1} f_\alpha^{eq}\xi_\alpha/\rho, \tag{S7}$$

$$\mathrm{w}_\alpha=\frac{1}{\sqrt{\pi}}\int e^{-\xi^2}\prod_{\substack{\beta=0\\ \beta\neq\alpha}}^{q-1}\frac{\xi-\xi_\beta}{\xi_\alpha-\xi_\beta}d\xi. \tag{S8}$$

Then all remained is to choose a $2n$-degree abscissa set or quadrature $\{\xi_0,\ldots,\xi_{q-1}\}$, which evaluates the integral exactly for $k\leq 2n$,

$$I^k=\int\frac{1}{\sqrt{\pi}}e^{-\xi^2}\xi^k d\xi=\sum_{\alpha=0}^{q-1}\mathrm{w}_\alpha\xi_\alpha^k. \tag{S9}$$

$\xi_\alpha$ is related to micro velocity $v_\alpha$ with $\xi_\alpha=v_\alpha/\sqrt{2RT}$. In practice, the classical LB algorithm of colliding on nodes and streaming along links requires that the quadrature $\{\xi_\alpha\}$ has the form $\{v_\alpha\}/\sqrt{2RT}$ where $v_\alpha$ is the integer-valued discrete micro velocity and $1/\sqrt{2RT}$ is a real-valued lattice constant.

## II. pGHQ THEORY

pGHQ is a generalization of the Gauss-Hermite quadrature. It can be stated as, given a $q$-point abscissa set $\{\xi_0,\ldots,\xi_{q-1}\}$, once its abscissa polynomial,

$$W_q(\xi)=\prod_{\alpha=0}^{q-1}(\xi-\xi_\alpha), \tag{S10}$$

satisfies the orthogonal relationship,

$$\int e^{-\xi^2}W_q(\xi)\,p(\xi)\,d\xi=0,\forall p(\xi)\in\mathbb{P}_{K(K<q)}, \tag{S11}$$

where $\mathbb{P}_K$ is the set of polynomials of degrees not exceeding $K$, it has $(q+K)$ quadrature degree. Once $K=q-1$, this is exactly the statement of the Gauss-Hermite quadrature. The prove of pGHQ is plain. For any $q$-point abscissa set $\{\xi_0,\ldots,\xi_{q-1}\}$, we can employ polynomial interpolation quadrature to generate weights $\{\mathrm{w}_\alpha\}$,

$$\mathrm{w}_\alpha=\frac{1}{\sqrt{\pi}}\int e^{-\xi^2}\prod_{\substack{\beta=0\\ \beta\neq\alpha}}^{q-1}\frac{\xi-\xi_\beta}{\xi_\alpha-\xi_\beta}d\xi, \tag{S12}$$

which fulfills all equations with $0\leq k<q$ ,

$$\int\frac{1}{\sqrt{\pi}}e^{-\xi^2}\xi^k d\xi=\sum_{\alpha=0}^{q-1}\mathrm{w}_\alpha\xi_\alpha^k, \tag{S13}$$

i.e. the $(q-1)$th quadrature equation system (QES) in paper. It should be noted that there is an extra coefficient $1/\sqrt{\pi}$ in above formulas which is specially designed for the extension of this justification in LB equilibrium distribution discretization. The formulas indicate that for any given polynomial of $\xi$ with degree not exceeding $(q-1)$, $f_{q-1}(\xi)$, the following equation is always satisfied,

$$\int\frac{1}{\sqrt{\pi}}e^{-\xi^2}f_{q-1}(\xi)\,d\xi=\sum_{\alpha=0}^{q}\mathrm{w}_\alpha f_{q-1}(\xi_\alpha). \tag{S14}$$

Now for $\xi^{q+l}$ where $l\leq K$, it can be expressed as

$$\xi^{q+l}=W_q(\xi)\,f_l(\xi)+p_{q-1}(\xi)\,, \tag{S15}$$

where $f_l(\xi)$ and $p_{q-1}(\xi)$ denote polynomials of $\xi$ with degree not exceeding $l$ and $(q-1)$ respectively. Due to the orthogonal relationship in Eq. (S11), the integral of $\xi^{q+l}$ reads

$$\int \frac{1}{\sqrt{\pi}} e^{-\xi^2} \xi^{q+l} d\xi = \int \frac{1}{\sqrt{\pi}} e^{-\xi^2} \left(W_q(\xi) f_l(\xi) + p_{q-1}(\xi)\right) d\xi = \int \frac{1}{\sqrt{\pi}} e^{-\xi^2} p_{q-1}(\xi) d\xi. \tag{S16}$$

As the abscissas are the zeros of abscissa polynomial, then the quadrature of $\xi^{q+l}$ yields

$$\sum_{\alpha=0}^{q-1} \mathrm{w}_\alpha \xi_\alpha^{q+l} = \sum_{\alpha=0}^{q-1} \mathrm{w}_\alpha \left(W_q(\xi_\alpha) f_l(\xi_\alpha) + p_{q-1}(\xi_\alpha)\right) = \sum_{\alpha=0}^{q-1} \mathrm{w}_\alpha p_{q-1}(\xi_\alpha). \tag{S17}$$

With relation in Eq. (S14), then quadrature equation (QE) with exponent $(q+l)$ in paper is satisfied,

$$\int \frac{1}{\sqrt{\pi}} e^{-\xi^2} \xi^{q+l} d\xi = \sum_{\alpha=0}^{q-1} \mathrm{w}_\alpha \xi_\alpha^{q+l}. \tag{S18}$$

As $l$ can be any integers below $K$, it indicates that once the orthogonal relationship in Eq. (S11) was established, the set $\{\xi_\alpha\}$ and the corresponding weights $\{\mathrm{w}_\alpha\}$ calculated by Eq. (S12) fulfill

$$\int \frac{1}{\sqrt{\pi}} e^{-\xi^2} \xi^{k} d\xi = \sum_{\alpha=0}^{q-1} \mathrm{w}_\alpha \xi_\alpha^{k}, \tag{S19}$$

for all $k \le q+K$, i.e. the $(q+K)$th QES. Hence the pGHQ theory is proven.

As the derivation shows, the kernel equation of pGHQ is the abscissa polynomial orthogonality in Eq. (S11). This relationship equals

$$W_q(\xi) = \sum_{i=K+1}^{q} A_i H_i(\xi), \tag{S20}$$

which indicates that the Hermite-polynomial-form expression of abscissa polynomial only contains Hermite polynomials with degree between $(K+1)$ and $q$. Here is the proof. For any polynomial, we can rewrite it in Hermite polynomials,

$$W_q(\xi) = \sum_{i=0}^{q} A_i H_i(\xi). \tag{S21}$$

The Hermite polynomials possess the following orthogonal property [2],

$$\int \frac{1}{\sqrt{\pi}} e^{-\xi^2} H_m(\xi) H_n(\xi) d\xi = 2^n n! \delta_{mn}. \tag{S22}$$

where $\delta_{mn}$ is the Kronecker delta. As the orthogonal relationship in Eq. (S11) indicates that $p(\xi)$ can be any polynomial with degree not exceeding $K$. Taking $p(\xi)$ as $\{H_0(\xi), H_1(\xi), ..., H_K(\xi)\}$, we can get

$$\int \frac{1}{\sqrt{\pi}} e^{-\xi^2} W_q(\xi) H_m(\xi) d\xi = 0, \tag{S23}$$

where $0 \le m \le K$. Employing the Hermite-polynomial-form abscissa polynomial and Hermite polynomial orthogonality, Eq. (S23) leads to

$$\int \frac{1}{\sqrt{\pi}} e^{-\xi^2} W_q(\xi) H_m(\xi) d\xi = \int \frac{1}{\sqrt{\pi}} e^{-\xi^2} \sum_{i=0}^{q} A_i H_i(\xi) H_m(\xi) d\xi = A_m 2^m m! = 0, \tag{S24}$$

for $0 \le m \le K$. Thus the equivalence between the original pGHQ orthogonal relationship Eq. (S11) and Hermite-polynomial form of abscissa polynomial Eq. (S20) is justified.

In discretization of LB equilibrium distribution, we employ the equivalent statement of pGHQ, that given a $q$-point abscissa set $\{\xi_0, \xi_1, ..., \xi_{q-1}\}$ who has $(q+K)\{K<q\}$ quadrature degree under weight function $e^{-\xi^2}$, its abscissa polynomial yields

$$W_q(\xi) = \prod_{\alpha=0}^{q-1}(\xi - \xi_\alpha) = \sum_{i=K+1}^{q} A_i H_i(\xi), \tag{S25}$$

i.e. the Hermite-polynomial form of abscissa polynomial only consists of Hermite polynomials with degree between $(K+1)$ and $q$. As the coefficient of $\xi^q$ in abscissa polynomial equals 1, we also can specify the coefficient of $H_q(\xi)$ as $A_q = 1/2^q$, which generates the orthogonality expression in paper,

$$W_q(\xi) = \sum_{i=K+1}^{q-1} A_i H_i(\xi) + \frac{1}{2^q} H_q(\xi). \tag{S26}$$

## III. MATHEMATICAL EQUIVALENCE BETWEEN THE pGHQ SCHEME AND THE SHAN SCHEME

Before we address the detailed relation between the pGHQ scheme and the Shan scheme[3], we would like to briefly revisit the theory of the Shan scheme. It worths noting that all derivation is based on 1-dimensional lattices. The Shan scheme employs the similar mathematical technique to turn the discretization into a quadrature problem with a different form of Hermite polynomials, probabilists' Hermite polynomials,

$$\begin{aligned} M^k &= \int \frac{\rho}{\sqrt{2\pi RT}} e^{-(v-u)^2/(2RT)} v^k dv \\ &= \left(\sqrt{RT}\right)^k \frac{\rho}{\sqrt{2\pi}} \int e^{-(\xi-\phi)^2/2} \xi^k d\xi \\ &= \left(\sqrt{RT}\right)^k \frac{\rho}{\sqrt{2\pi}} \int e^{-\xi^2/2} \sum_{i=0}^{\infty} He_i(\xi) \frac{\phi^i}{i!} \xi^k d\xi \\ &= \left(\sqrt{RT}\right)^k \sum_{\alpha=0}^{q-1} f_\alpha^{eq} \xi_\alpha^k, \end{aligned} \tag{S27}$$

where $v$ and $u$ stand for micro and macro velocity respectively, $T$ is the temperature , $\rho$ is the density, $R$ is the gas constant, $\xi$ and $\phi$ stand for corresponding dimensionless micro and macro velocity with relation $\xi = v/\sqrt{RT}$ and $\phi = u/\sqrt{RT}$. Since the Hermite polynomials $He_i(\xi)$ with degree above $k$ has no influence on the calculation of $k$-th moment integral $M^k$ due to the orthogonality, the $n$ moment degree discretization turns into finding a set of abscissas $\{\xi_\alpha\}$ and their corresponding weights $\{\mathrm{w}_\alpha\}$ who has at least $2n$ quadrature degree. The discretized equilibrium distribution reads

$$f_\alpha^{eq} = \mathrm{w}_\alpha \rho \sum_{i=0}^{n} He_i(\xi_\alpha) \frac{\phi^i}{i!}, \tag{S28}$$

with

$$\rho = \sum_{\alpha=0}^{q-1} f_\alpha^{eq}, \quad \phi = \sum_{\alpha=0}^{q-1} f_\alpha^{eq} \xi_\alpha / \rho. \tag{S29}$$

And the abscissas $\{\xi_\alpha\}$ and weights $\{\mathrm{w}_\alpha\}$ satisfy

$$\frac{1}{\sqrt{2\pi}} \int e^{-\xi^2/2} \xi^k d\xi = \sum_{\alpha=0}^{q-1} \mathrm{w}_\alpha \xi_\alpha^k, \tag{S30}$$

for all $0 \leq k \leq 2n$. Employing the orthogonality of Hermite polynomials,

$$\frac{1}{\sqrt{2\pi}} \int e^{-\xi^2/2} He_k(\xi) d\xi = \begin{cases} 1 & k=0 \\ 0 & k>0 \end{cases}, \tag{S31}$$

and the polynomial relationship,

$$\xi^k = k! \sum_{m=0}^{\lfloor k/2 \rfloor} \frac{1}{2^m m! \, (k-2m)!} He_{k-2m}(\xi), \tag{S32}$$

then the left-hand side of Eq. (S30) yields

$$\frac{1}{\sqrt{2\pi}} \int e^{-\frac{\xi^2}{2}} \xi^k d\xi = \begin{cases} \frac{(2i)!}{2^i i!} & k = 2i \\ 0 & k = 2i+1 \end{cases}. \tag{S33}$$

Hence the constraint equations of abscissas $\{\xi_\alpha\}$ and weights $\{\mathrm{w}_\alpha\}$ for $n$ moment degree discretization are

$$\sum_{\alpha=0}^{q-1} \mathrm{w}_\alpha \xi_\alpha^k = \begin{cases} \frac{(2i)!}{2^i i!} & k = 2i \\ 0 & k = 2i+1 \end{cases}, \tag{S34}$$

where $0 \le k \le 2n$. The streaming-on-mesh algorithm of LB method requires the abscissas have the form,

$$\xi_\alpha = v_\alpha c, \tag{S35}$$

where $c$ is real-valued lattice constant and $v_\alpha$ integer-valued discrete velocity. It worths noting that, due to the different form of employed Hermite polynomials, the expression of lattice constant $c$ is $c = 1/\sqrt{RT}$ instead of $c = 1/\sqrt{2RT}$ in pGHQ scheme.

Now the question is how to solve the constraint equations in Eq. (S34). The Shan scheme gives a procedure for minimal **compact** symmetrical lattices on range $[-5, 5]$. The idea is quite simple, given a moment degree $(2n+1)$, trying to eliminate weights $\mathrm{w}_\alpha$ on range $\{0, \pm1, ..., \pm n\}$ as many as possible by tuning lattice constant $c$. To make the derivation generic, we employ a general $(2n+1)$-point abscissa set without predefined symmetric form in the Shan scheme, $\{v_0, v_1, ...v_{2n}\}c$. The first step of the Shan scheme is to construct an equation matrix for this lattices,

$$\sum_{\alpha=0}^{2n} (v_\alpha c)^k \mathrm{w}_\alpha = m^k, \tag{S36}$$

where $0 \le k \le 2n$ and

$$m^k = \frac{1}{\sqrt{2\pi}} \int e^{-\frac{\xi^2}{2}} \xi^k d\xi.$$

Then the Shan scheme solves this equation system to obtain the expression of weights $\{\mathrm{w}_\alpha\}$, which are univariate polynomials of lattice constant $c$. In fact, this procedure can be formularized. Employing the first $2n$ abscissas, we construct a polynomial expression for $\xi^{2n}$,

$$\xi^{2n} = \prod_{\alpha=0}^{2n-1} (\xi - v_\alpha c) + P_{2n-1}(\xi), \tag{S37}$$

then the left-hand side of $k = 2n$ equation in Shan's equation matrix reads

$$\sum_{\alpha=0}^{2n} (v_\alpha c)^{2n} \mathrm{w}_\alpha = \sum_{\alpha=0}^{2n} \left( \prod_{\beta=0}^{2n-1} (v_\alpha c - v_\beta c) + P_{2n-1}(v_\alpha c) \right) \mathrm{w}_\alpha = \sum_{\alpha=0}^{2n} P_{2n-1}(v_\alpha c) \mathrm{w}_\alpha + \mathrm{w}_{2n} \prod_{\alpha=0}^{2n-1} (v_{2n} - v_\alpha) c, \tag{S38}$$

and the right-hand side leads to

$$m^{2n} = \frac{1}{\sqrt{2\pi}} \int e^{-\frac{\xi^2}{2}} \left( \prod_{\alpha=0}^{2n-1} (\xi - v_\alpha c) + P_{2n-1}(\xi) \right) d\xi. \tag{S39}$$

Since the identity of $k = 2n$ equation is meaningful if and only if all $k = \{0, ..., 2n-1\}$ ones satisfy, which ensures

$$\sum_{\alpha=0}^{2n} P_{2n-1}(v_\alpha c) \mathrm{w}_\alpha = \frac{1}{\sqrt{2\pi}} \int e^{-\frac{\xi^2}{2}} P_{2n-1}(\xi) d\xi, \tag{S40}$$

then the formula for $\mathrm{w}_{2n}$ is

$$\mathrm{w}_{2n} = \frac{\frac{1}{\sqrt{2\pi}} \int e^{-\frac{\xi^2}{2}} \prod_{\alpha=0}^{2n-1} (\xi - v_\alpha c) d\xi}{\prod_{\alpha=0}^{2n-1} (v_{2n} - v_\alpha) c}. \tag{S41}$$

The derivation is independent from detailed sequence of abscissa set $\{v_0, v_1, ... v_{2n}\}c$, thus we can extend Eq. (S41) into arbitrary $\mathrm{w}_\alpha$ in the same equation matrix,

$$\mathrm{w}_\alpha = \frac{\frac{1}{\sqrt{2\pi}} \int e^{-\frac{\xi^2}{2}} \prod_{\beta=0,\beta\neq\alpha}^{2n} (\xi - v_\beta c) d\xi}{\prod_{\beta=0,\beta\neq\alpha}^{2n} (v_\alpha - v_\beta) c}. \tag{S42}$$

It is the formula of polynomial interpolation quadrature to generate weights for abscissa set $\{v_0, v_1, ... v_{2n}\}c$. Now we try to eliminate $\{\mathrm{w}_\alpha\}$ to make the abscissa set minimal through tuning the lattice constant $c$. Here eliminating $\mathrm{w}_l$ is taken as an instance. Before starting derivation, we construct an abscissa polynomial with the un-eliminated abscissas,

$$W_{2n}(\xi) = \prod_{\alpha=0,\alpha\neq l}^{2n} (\xi - v_\alpha c). \tag{S43}$$

Then the formula of weight $\mathrm{w}_l$ can be expressed as

$$\mathrm{w}_l = \frac{\frac{1}{\sqrt{2\pi}} \int e^{-\frac{\xi^2}{2}} W_{2n}(\xi) d\xi}{W_{2n}(v_l c)}. \tag{S44}$$

Since $W_{2n}(v_l c) \neq 0$, then $\mathrm{w}_l = 0$ leads to

$$\frac{1}{\sqrt{2\pi}} \int e^{-\frac{\xi^2}{2}} W_{2n}(\xi) d\xi = 0. \tag{S45}$$

Employing the Hermite-polynomial-form abscissa polynomial,

$$W_{2n}(\xi) = \sum_{i=0}^{2n} A_i He_i(\xi), \tag{S46}$$

Eq. (S45) equals,

$$\frac{1}{\sqrt{2\pi}} \int e^{-\frac{\xi^2}{2}} W_{2n}(\xi) d\xi = \frac{1}{\sqrt{2\pi}} \int e^{-\frac{\xi^2}{2}} \sum_{i=0}^{2n} A_i He_i(\xi) d\xi = \frac{1}{\sqrt{2\pi}} \int e^{-\frac{\xi^2}{2}} A_0 He_0(\xi) d\xi = A_0 = 0 \tag{S47}$$

And the un-eliminated weights $\mathrm{w}_\alpha$ can be simplified as

$$\begin{aligned}
\mathrm{w}_\alpha &= \frac{\frac{1}{\sqrt{2\pi}} \int e^{-\frac{\xi^2}{2}} \prod_{\beta=0,\beta\neq\alpha}^{2n} (\xi - v_\beta c) d\xi}{\prod_{\beta=0,\beta\neq\alpha}^{2n} (v_\alpha - v_\beta) c} \\
&= \frac{\frac{1}{\sqrt{2\pi}} \int e^{-\frac{\xi^2}{2}} \left( W_{2n}(\xi) + \prod_{\beta=0,\beta\neq\alpha,\beta\neq l}^{2n} (\xi - v_\beta c)(v_\alpha c - v_l c) \right) d\xi}{(v_\alpha - v_l) c \prod_{\beta=0,\beta\neq\alpha,\beta\neq l}^{2n} (v_\alpha - v_\beta) c} \\
&= \frac{\frac{1}{\sqrt{2\pi}} \int e^{-\frac{\xi^2}{2}} \prod_{\beta=0,\beta\neq\alpha,\beta\neq l}^{2n} (\xi - v_\beta c) d\xi}{\prod_{\beta=0,\beta\neq\alpha,\beta\neq l}^{2n} (v_\alpha - v_\beta) c}.
\end{aligned} \tag{S48}$$

It is the weight formula of polynomial interpolation quadrature for un-eliminated abscissas. This derivation can be directly extended into multiple elimination of $\{w_\alpha\}$. For an example, we eliminate $K$ points from the abscissa set $\{v_0, v_1, ...v_{2n}\}c$. Denoting the eliminated points as $\{e_0, e_1, ...e_{K-1}\}c$ and remained points as $\{r_0, r_1, ...r_{2n-K}\}c$, then we can construct their abscissa polynomials,

$$E_K(\xi) = \prod_{\alpha=0}^{K-1} (\xi - e_\alpha c), \tag{S49}$$

$$R_{2n-K+1}(\xi) = \prod_{\alpha=0}^{2n-K} (\xi - r_\alpha c). \tag{S50}$$

Therefore the weight expression of eliminated points can be expressed as,

$$\mathrm{w}_\alpha = \frac{\frac{1}{\sqrt{2\pi}} \int e^{-\frac{\xi^2}{2}} R_{2n-K+1}(\xi) \frac{E_K(\xi)}{\xi - v_\alpha c} d\xi}{R_{2n-K+1}(v_\alpha c) \frac{E_K(v_\alpha c)}{v_\alpha c - v_\alpha c}}. \tag{S51}$$

As we discussed in the single elimination that the denominator in the above expression cannot be 0, then the elimination of $\mathrm{w}_\alpha$ equals,

$$\frac{1}{\sqrt{2\pi}} \int e^{-\frac{\xi^2}{2}} R_{2n-K+1}(\xi) \frac{E_K(\xi)}{\xi - v_\alpha c} d\xi = 0 \tag{S52}$$

for $v_\alpha \in \{e_0, e_1, ...e_{K-1}\}$. Implementing simple algebraic operations on above equations, we can construct series of equations,

$$\frac{1}{\sqrt{2\pi}} \int e^{-\frac{\xi^2}{2}} R_{2n-K+1}(\xi) He_k(\xi) d\xi = 0 \tag{S53}$$

for $0 \le k < K$. These two equation systems, Eq. (S52) and Eq. (S53), are mathematically equivalent for lattice constant $c$. Introducing the Hermite polynomial form of $R_{2n-K+1}(\xi)$,

$$R_{2n-K+1}(\xi) = \sum_{i=0}^{2n-K+1} A_i He_i(\xi), \tag{S54}$$

and the orthogonal relationship among Hermite polynomials,

$$\frac{1}{\sqrt{2\pi}} \int e^{-\frac{\xi^2}{2}} He_n(\xi) He_m(\xi) d\xi = n!\delta_{nm}, \tag{S55}$$

the obtained series of Eq. (S53) can be written as,

$$\frac{1}{\sqrt{2\pi}} \int e^{-\frac{\xi^2}{2}} R_{2n-K+1}(\xi) He_k(\xi) d\xi = \frac{1}{\sqrt{2\pi}} \int e^{-\frac{\xi^2}{2}} \sum_{i=0}^{2n-K+1} A_i He_i(\xi) He_k(\xi) d\xi = A_k k! = 0, \tag{S56}$$

for $0 \le k < K$. Hence the elimination of points equals setting the corresponding Hermite polynomial coefficients in abscissa polynomial to 0 through tuning the lattice constant $c$, which is exactly the approach of the pGHQ scheme. Now we re-evaluate the weight formulas for the un-eliminated points. With the help of Eq. (S52), the numerator of un-eliminated $\mathrm{w}_\alpha$ can be transformed into,

$$\begin{aligned} \frac{1}{\sqrt{2\pi}} \int e^{-\frac{\xi^2}{2}} E_K(\xi) \frac{R_{2n-K+1}(\xi)}{\xi - v_\alpha c} d\xi &= \frac{1}{\sqrt{2\pi}} \int e^{-\frac{\xi^2}{2}} E_K(\xi) \left( \frac{\xi - v_\alpha c}{\xi - v_\beta c} + \frac{v_\alpha c - v_\beta c}{\xi - v_\beta c} \right) \frac{R_{2n-K+1}(\xi)}{\xi - v_\alpha c} d\xi, \\ &= \frac{1}{\sqrt{2\pi}} \int e^{-\frac{\xi^2}{2}} E_K(\xi) \frac{v_\alpha c - v_\beta c}{\xi - v_\beta c} \frac{R_{2n-K+1}(\xi)}{\xi - v_\alpha c} d\xi, \end{aligned} \tag{S57}$$

where $v_\beta \in \{e_0, e_1, ...e_{K-1}\}$ is an arbitrary eliminated point. This transformation can go on until we reach,

$$\begin{aligned} \frac{1}{\sqrt{2\pi}} \int e^{-\frac{\xi^2}{2}} E_K(\xi) \frac{R_{2n-K+1}(\xi)}{\xi - v_\alpha c} d\xi &= \frac{1}{\sqrt{2\pi}} \int e^{-\frac{\xi^2}{2}} E_K(\xi) \frac{E_K(v_\alpha c)}{E_K(\xi)} \frac{R_{2n-K+1}(\xi)}{\xi - v_\alpha c} d\xi, \\ &= \frac{E_K(v_\alpha c)}{\sqrt{2\pi}} \int e^{-\frac{\xi^2}{2}} \frac{R_{2n-K+1}(\xi)}{\xi - v_\alpha c} d\xi. \end{aligned} \tag{S58}$$

Therefore the un-eliminated $\mathrm{w}_\alpha$ leads to,

$$\mathrm{w}_\alpha = \frac{\frac{1}{\sqrt{2\pi}}\int e^{-\frac{\xi^2}{2}}\frac{R_{2n-K+1}(\xi)}{\xi - v_\alpha c}d\xi}{\frac{R_{2n-K+1}(v_\alpha c)}{v_\alpha c - v_\alpha c}}. \tag{S59}$$

This is the formula of polynomial interpolation quadrature for un-eliminated abscissas. Hence the matrix solving and point elimination in the Shan scheme can be directly replaced with the techniques in pGHQ scheme, i.e. solving the Hermite polynomial coefficient equations, which would significantly simplify the algorithm. As the Shan scheme employs probabilists' Hermite polynomial meanwhile pGHQ scheme uses physicists' Hermite polynomial, there is one last question need to be answered whether these two schemes are mathematically equivalent. Here we examine the their values of lattice constant $c$. As their lattice constant expressions are different, which are $c = 1/\sqrt{2RT}$ in the pGHQ scheme and $c = 1/\sqrt{RT}$ in the Shan scheme respectively, we would identify the value of $RT$. As we previously derived that both the pGHQ scheme and the Shan scheme can get the lattice constant value through solving the coefficient equations of abscissa polynomial, we start with the abscissa polynomial of the Shan scheme,

$$W_q(\xi) = \prod_{\alpha=0}^{q-1}(\xi - \xi_\alpha) = \sum_{i=0}^{q} A_i He_i(\xi). \tag{S60}$$

This equation is related to the micro velocity $v$ and its discrete velocity $v_\alpha$ as,

$$W_q(\xi) = \prod_{\alpha=0}^{q-1}(\xi - \xi_\alpha) = \left(\frac{1}{\sqrt{RT}}\right)^q \prod_{\alpha=0}^{q-1}(v - v_\alpha). \tag{S61}$$

Therefore the Hermite form of Shan abscissa polynomial equals,

$$W_q(\xi) = \sum_{i=0}^{q} A_i He_i\left(\frac{v}{\sqrt{RT}}\right) = \left(\frac{1}{\sqrt{RT}}\right)^q \prod_{\alpha=0}^{q-1}(v - v_\alpha). \tag{S62}$$

As the probabilists' Hermite polynomial can be expressed with physicists' Hermite polynomial as,

$$He_i(x) = 2^{-i/2} H_i\left(\frac{x}{\sqrt{2}}\right), \tag{S63}$$

then the Shan abscissa polynomial in physicists' Hermite polynomials reads,

$$W_q(\xi) = \sum_{i=0}^{q} A_i He_i\left(\frac{v}{\sqrt{RT}}\right) = \sum_{i=0}^{q} A_i 2^{-i/2} H_i\left(\frac{v}{\sqrt{2RT}}\right). \tag{S64}$$

Multiplying the equation Eq. (S64) with $2^{-q/2}$, we can obtain,

$$2^{-q/2} W_q(\xi) = \left(\frac{1}{\sqrt{2RT}}\right)^q \prod_{\alpha=0}^{q-1}(v - v_\alpha) = \sum_{i=0}^{q} A_i 2^{-(i+q)/2} H_i\left(\frac{v}{\sqrt{2RT}}\right). \tag{S65}$$

Its left hand side is the expression of pGHQ abscissa polynomial, which can be expressed as,

$$W_q^{pGHQ}(\xi) = \left(\frac{1}{\sqrt{2RT}}\right)^q \prod_{\alpha=0}^{q-1}(v - v_\alpha) = \sum_{i=0}^{q} A_i^{pGHQ} H_i\left(\frac{v}{\sqrt{2RT}}\right). \tag{S66}$$

As the expansion of a polynomial under physicists' Hermite polynomials is unique, then we can get,

$$A_i 2^{-(i+q)/2} = A_i^{pGHQ}. \tag{S67}$$

Hence $A_i$ and $A_i^{pGHQ}$ are mathematically equivalent equations for $RT$. Therefore we justify the equivalence between the pGHQ scheme and the Shan scheme.

As a conclusion, we prove that the Shan scheme and the pGHQ scheme are mathematically equivalent for unidimensional equilibrium distribution discretization. It should be noted that in this justification we use formulas to simplify the calculation of weights $\mathrm{w}_\alpha$ which in original version is computed through tediously solving the equation system of Eq. (S34) and extend the Shan's algorithm of predefined symmetric lattices into a general form. Even though, the modified Shan scheme is still more complicated than the pGHQ scheme.

## IV. MATHEMATICAL EQUIVALENCE BETWEEN pGHQ AND THE KARLIN-ASINARI SCHEME

The Karlin-Asinari scheme[4] is based on an observation that for a $q$-point discrete velocity set $\{v_\alpha\}$, there is a linear relation with constant coefficients $a_k$,

$$v^q = \sum_{k=0}^{q-1} a_k v^k, \tag{S68}$$

which applies to all velocities in this set. This linear relation prohibits the accurate evaluation of Maxwellian moment integral with degree $q$ ,

$$M^q = \int \frac{\rho}{\sqrt{\pi 2RT}} e^{-\frac{(v-u)^2}{2RT}} v^q dv \neq \sum_{\alpha=0}^{q-1} f_\alpha^{eq} v_\alpha^q, \tag{S69}$$

as the rightest term of the equation can be expressed,

$$\sum_{\alpha=0}^{q-1} f_\alpha^{eq} v_\alpha^q = \sum_{\alpha=0}^{q-1} f_\alpha^{eq} \sum_{k=0}^{q-1} a_k v_\alpha^k = \sum_{k=0}^{q-1} a_k M^k. \tag{S70}$$

The reason is plain, we cannot use Maxwellian moment integrals with degree below $q$ to construct $M^q$. The obtaining of the linear relation in the Karlin-Asinari scheme is quite clumsy, as they manually solve the coefficients $a_k$ through a linear system. Actually it can be directly constructed by setting the lattice polynomial $l_q(v)$ to 0,

$$l_q(v) = \prod_{\alpha=0}^{q-1} (v - v_\alpha) = 0. \tag{S71}$$

Therefore the deviation between the analytical and the evaluated Maxwellian moment integral with degree $q$ yields,

$$M^q - \sum_{\alpha=0}^{q-1} f_\alpha^{eq} v_\alpha^q = \int \frac{\rho}{\sqrt{\pi 2RT}} e^{-\frac{(v-u)^2}{2RT}} l_q(v)\, dv. \tag{S72}$$

Nondimensionalizing this equation with variables $\xi = v/\sqrt{2RT}$, $\phi = u/\sqrt{2RT}$, it leads to,

$$M^q - \sum_{\alpha=0}^{q-1} f_\alpha^{eq} v_\alpha^q = \left(\sqrt{2RT}\right)^q \int g W_q(\xi)\, d\xi, \tag{S73}$$

where $g$ is the dimensionless Maxwell distribution, $W_q(\xi)$ is the abscissa polynomial corresponding to the pGHQ scheme,

$$g = \frac{\rho}{\sqrt{\pi}} e^{-(\xi-\phi)^2}, \tag{S74}$$

$$W_q(\xi) = \prod_{\alpha=0}^{q-1} (\xi - \xi_\alpha) = \prod_{\alpha=0}^{q-1} \left(\frac{v}{\sqrt{2RT}} - \frac{v_\alpha}{\sqrt{2RT}}\right) = \left(\frac{1}{\sqrt{2RT}}\right)^q l_q(v). \tag{S75}$$

Employing their Hermite polynomial forms,

$$g = \frac{\rho}{\sqrt{\pi}} e^{-\xi^2} \sum_{i=0}^{\infty} H_i(\xi) \frac{\phi^i}{i!}, \tag{S76}$$

$$W_q(\xi) = \sum_{i=0}^{q} A_i H_i(\xi), \tag{S77}$$

the deviation equation reads,

$$M^q - \sum_{\alpha=0}^{q-1} f_\alpha^{eq} v_\alpha^q = \left(\sqrt{2RT}\right)^q \int \frac{\rho}{\sqrt{\pi}} e^{-\xi^2} \sum_{i=0}^{\infty} H_i(\xi) \frac{\phi^i}{i!} \sum_{i=0}^{q} A_i H_i(\xi) d\xi = \rho \sum_{i=0}^{q} \left(\sqrt{2RT}\right)^{q-i} A_i 2^i u^i. \tag{S78}$$

The Karlin-Asinari scheme proposed that one can eliminate the deviation on selected $u^i$ terms by tuning the value of $RT$, i.e. solving equation $\left(\sqrt{2RT}\right)^{q-i} A_i 2^i = 0$. It should be noted that in their paper notation $RT$ is simplified as reference temperature $T_0$. They proposed the match closure which eliminate the deviation of term $u^1$. Since $RT$ cannot be zero, the equation is equal to $A_1 = 0$ which is exactly the Hermite coefficient equation in the pGHQ scheme. As the symmetric discrete velocity set $\{0, \pm v_1, \cdots, \pm v_{n-1}\}$ predefined in the Karlin-Asinari scheme ensures that its abscissa polynomial of Hermite polynomial form only involves Hermite polynomials with odd degree,

$$W_{2n-1}(\xi) = \xi \prod_{\alpha=0}^{n-1} \left(\xi^2 - \xi_\alpha^2\right) = \sum_{i=0}^{n-1} A_{2i+1} H_{2i+1}(\xi), \tag{S79}$$

the Karlin-Asinari scheme can be regarded as solving the $(2n-1) \sim 2^{th}$ HCES in the pGHQ scheme. And pGHQ can be taken as the generalization of the Karlin-Asinari scheme including asymmetric lattices or other $u^i$ terms with a concise algorithm. pGHQ avoids the calculation of Eq. (S78) by directly analyzing the Hermite polynomial form of the abscissa polynomial in Eq. (S77).

The Karlin-Asinari scheme also involves the calculation of weights. Given a discrete velocity set $\{v_0, v_1, v_{q-1}\}$ with a real-valued solution of $RT$, it employs the Maxwell moment integrals at $u = 0$ to calculate them, which read,

$$\int \frac{\rho}{\sqrt{2RT\pi}} e^{-\frac{v^2}{2RT}} v^k dv = \rho \sum_{\alpha=0}^{q-1} \mathrm{w}_\alpha v_\alpha^k, \tag{S80}$$

where $k < q$. Nondimensionalizing velocity $v$ as $\xi = v/\sqrt{2RT}$, this equation system is exactly the $(q-1)$th QES with an extra coefficient $\rho$,

$$\int \frac{\rho}{\sqrt{\pi}} e^{-\xi^2} \xi^k d\xi = \rho \sum_{\alpha=0}^{q-1} \mathrm{w}_\alpha \xi_\alpha^k, \tag{S81}$$

for $k < q$. As shown in the pGHQ theory derivation, the polynomial interpolation quadrature offers a formula to obtain these weights,

$$\mathrm{w}_\alpha = \frac{1}{\sqrt{\pi}} \int e^{-\xi^2} \prod_{\substack{\beta=0 \\ \beta\neq\alpha}}^{q-1} \frac{\xi - \xi_\beta}{\xi_\alpha - \xi_\beta} d\xi, \tag{S82}$$

which is also the formula for the pGHQ weights. Hence the tedious equation system solving for weights in the Karlin-Asinari scheme can be replaced by pGHQ weight formula.

To conclude, we mathematically justify that the solving of $RT$ and weights in the Karlin-Asinari scheme can be replaced by the concise algorithm of the pGHQ scheme though their constructions of $f_\alpha^{eq}$ are different. And pGHQ can be regarded as the general form of the mathematical mechanism behind the Karlin-Asinari scheme.


[1] X. W. Shan and X. Y. He, Phys. Rev. Lett. **80**, 65 (1998).

[2] G. B. Arfken, H. J. Weber, and F. E. Harris, *Mathematical Methods for Physicists: A Comprehensive Guide* (Academic Press, 2011).

[3] X. Shan, J. Comput. Sci.-Neth. **17**, 475 (2016).

[4] I. Karlin and P. Asinari, Physica A **389**, 1530 (2010).
